# Supplementary material for: SPIRT: A Fault-Tolerant and Reliable Peer-to-Peer Serverless ML Training Architecture
Source: arXiv:2309.14148 source file (2023-09-25)
Supplement: Supplementary file 1 [file Appendix.tex]

\appendix

\setcounter{figure}{0}
\begin{figure}[htp]
  \centering 
  \includegraphics[scale=.8]{boxplots.png}
  \caption{Github VR projects properties} \label{Figure:GitHubProperties}
\end{figure}
